# Supplementary material for: Origins of suppressed self-diffusion of nanoscale constituents of a complex liquid
Source: arXiv:2404.17756 ancillary file (2026-11-07)
Supplement: Supplementary file 1 [file SI.pdf]

# Supporting Information for Origins of suppressed self-diffusion of nanoscale constituents of a complex liquid

Christian P. N. Tanner,<sup>†</sup> Vivian R. K. Wall,<sup>†</sup> Mumtaz Gababa,<sup>†</sup> Joshua Portner,<sup>‡</sup> Ahhyun Jeong,<sup>‡</sup> Matthew J. Hurley,<sup>¶,§</sup> Nicholas Leonard,<sup>¶</sup> Jonathan G. Raybin,<sup>†</sup> James K. Utterback,<sup>†,||</sup> Ahyoung Kim,<sup>†,⊥</sup> Andrei Fluerașu,<sup>#</sup> Yanwen Sun,<sup>@</sup> Johannes Möller,<sup>△</sup> Alexey Zozulya,<sup>△</sup> Wonhyuk Jo,<sup>△</sup> Felix Brausse,<sup>△</sup> James Wrigley,<sup>△</sup> Ulrike Boesenberg,<sup>△</sup> Wei Lu,<sup>△</sup> Roman Shayduk,<sup>△</sup> Mohamed Youssef,<sup>△</sup> Anders Madsen,<sup>△</sup> David T. Limmer,<sup>†,▽,††</sup> Dmitri V. Talapin,<sup>‡,‡‡</sup> Samuel W. Teitelbaum,<sup>¶</sup> and Naomi S. Ginsberg<sup>\*,†,¶,§§,|||,††,⊥⊥</sup>

<sup>†</sup>*Department of Chemistry, University of California, Berkeley, CA 94720, USA*

<sup>‡</sup>*Department of Chemistry, James Franck Institute, and Pritzker School of Molecular Engineering, University of Chicago, Chicago, IL 60637, USA*

<sup>¶</sup>*Department of Physics, Arizona State University, Tempe, AZ 85287, USA*

<sup>§</sup>*Present Address: Department of Physics, Stanford University, Stanford, CA 94305, USA*

<sup>||</sup>*Present Address: Sorbonne Université, CNRS, Institut des NanoSciences de Paris, INSP, 75005 Paris, France*

<sup>⊥</sup>*Present Address: California Institute of Technology, Pasadena, CA 91125, USA*

<sup>#</sup>*Brookhaven National Laboratory, NSLS-II, Upton, NY 11973, USA*

<sup>@</sup>*Linac Coherent Light Source, SLAC National Accelerator Laboratory, Menlo Park, CA 94025, USA*

<sup>△</sup>*European X-ray Free-Electron Laser Facility, Holzkoppel 4, 22869 Schenefeld, Germany*

<sup>▽</sup>*Chemical Sciences and Materials Sciences Divisions, Lawrence Berkeley National Laboratory, Berkeley, CA 94720, USA*

<sup>††</sup>*Kavli Energy NanoSciences Institute, University of California, Berkeley, CA 94720, USA*

<sup>‡‡</sup>*Center for Nanoscale Materials, Argonne National Laboratory, Argonne, IL 60517, USA*

<sup>¶¶</sup>*Department of Physics, University of California, Berkeley, CA 94720, USA*

<sup>§§</sup>*Molecular Biophysics and Integrated Bioimaging Division, Lawrence Berkeley National Laboratory, Berkeley, CA 94720, USA*

<sup>|||</sup>*Materials Sciences and Chemical Sciences Division, Lawrence Berkeley National Laboratory, Berkeley, CA 94720, USA*

<sup>⊥⊥</sup>*STROBE, NSF Science & Technology Center, Berkeley, CA 94720, USA*

E-mail: nsginsberg@berkeley.edu

# Methods

**Sample preparation.** Stock solutions of  $5.8 \pm 0.3$  nm PbS NCs with  $\text{Sn}_2\text{S}_6^{4-}$  ligands in N-methylformamide (NMF) and solutions of 0.5 M  $\text{K}_3\text{AsS}_4$  salt in NMF were prepared following a procedure previously outlined[6, 20]. In a nitrogen filled glovebox,  $\sim 50$   $\mu\text{L}$  of a solution of 5.8 nm PbS NCs with  $\text{Sn}_2\text{S}_6^{4-}$  ligands in mixtures of NMF and N,N-dimethylformamide (DMF) at volume fractions of  $\sim 0.001$  to 0.02 with varying amounts of  $\text{K}_3\text{AsS}_4$  salt were loaded into 0.9 mm outer-diameter borosilicate glass capillaries with 20-micron-thick walls. The capillaries were sealed and transported to the beamline for measurement.

**SAXS/XPCS experiments.** All SAXS/XPCS data were collected at the Materials Imaging and Dynamics (MID) instrument at the European XFEL. The X-ray photon energy was 12.3 keV and the sample-to-detector distance was 7 m. The X-ray beam size was  $\sim 2\text{-}3$   $\mu\text{m}$  (**Figure S7**) and typical X-ray pulse energies at the sample position were  $\sim 2\text{-}3$   $\mu\text{J}$ . Capillaries of PbS NCs at various concentrations dissolved in mixtures of NMF and DMF with varying amounts of  $\text{K}_3\text{AsS}_4$  salt were mounted at the beamline for data collection. The XFEL produced trains of ultrafast ( $\sim 50$  fs) spatially coherent X-ray pulses at a rate of 2.2 MHz. Each pulse train had 50 pulses. The first pulse of each train is delivered 0.1 s after the first pulse of the previous pulse train. Two-dimensional X-ray scattering data were collected on the AGIPD and azimuthally integrated to obtain one-dimensional X-ray scattering patterns,  $I(q)$ .

**Modelling of SAXS patterns.** We model the background-subtracted scattered intensity as  $I(q) = I_{\text{colloid}}(q) + I_{\text{liquid}}(q)$ , where  $I_{\text{colloid}}(q)$  is the scattered intensity from dilute, polydisperse, hard spheres and  $I_{\text{liquid}}(q)$  is the scattered intensity from finite-sized liquid clusters of hard spheres.[19, 20]  $I_{\text{colloid}}(q)$  is given by  $P(q)$ , the form factor for hard spheres of radius  $R$ , and has the explicit form  $P(q, R, \Delta R, c_1) = c_1 \int_0^\infty |F(q, R)|^2 V(R)^2 \tilde{P}(R, \Delta R) dR$ , where  $F(q, R) = 3[\sin(qR) - qR \cos(qR)]/(qR)^3$ ,  $V(R)$  is the volume of the hard sphere,  $\tilde{P}(R, \Delta R)$  is a Gaussian probability distribution centered at  $R$  with standard deviation  $\Delta R$ , and  $c_1$  is a value directly proportional to the number of hard spheres. For the liquid phase,  $I_{\text{liquid}}(q) = P(q)S_{\text{liquid}}(q)$ , where  $S_{\text{liquid}}(q)$  is given by the solution to the Ornstein-Zernike equation using the Percus-Yevick closure relation for the case of hard spheres[16, 23, 12] plus an additional  $q^{-4}$  term to describe the scattering at low  $q$ . To explicitly compute  $I_{\text{colloid}}(q)$  and  $I_{\text{liquid}}(q)$  we use xrsdkit (<https://github.com/scattering-central/xrsdkit>).

**Structure factor extraction.** To extract  $S^c(q)$  from the experimentally measured SAXS patterns, we divide  $I(q)$  by the best-fit  $P(q)$  function (green curve in **Figure 2b** in the main text). We obtain a good estimate for  $S^\ell(q)$  based on the fit to the SAXS pattern in **Figure 2b** in the main text. These structure factors are corrected for polydispersity by first subtracting  $(1 - X_p(q))$  and then dividing by  $X_p(q)$ , where  $X_p(q) = \frac{[\int_0^\infty dR \tilde{P}(R, \Delta R) F(q, R) V(R)]^2}{P(q) \int_0^\infty dR \tilde{P}(R, \Delta R) V(R)^2}$  is the decoupling amplitude.[24] The decoupling amplitude is shown in **Figure S5**.

**Correlation analysis.** Two-time correlation functions are defined via  $C_n(q, t_1, t_2) = \frac{\langle \delta I_n(q, t_1) \delta I_n(q, t_2) \rangle_{\text{sp}}}{\langle I_n(q, t_1) \rangle_{\text{sp}} \langle I_n(q, t_2) \rangle_{\text{sp}}}$ , where  $\delta I_n(q, t_1) = I_n(q, t_1) - \langle I_n(q, t_1) \rangle_{\text{sp}}$ ,  $\langle \dots \rangle_{\text{sp}}$  denotes an average over speckles in the same region of interest on the detector corresponding to the value of  $q$ , and  $I_n(q, t_1)$  and  $I_n(q, t_2)$  denote the scattered intensity in pulse train  $n$  as a function of times  $t_1$  and  $t_2$ , which take on values from 0 to 22.15  $\mu\text{s}$  (the duration of a single pulse train). The parameter  $n$  is the index of the pulse train, which goes from 1 to  $N$ , where  $N$  is the total

number of pulse trains in a measurement.  $C(q, t_1, t_2, n)$  is calculated for each pulse train,  $n$ , in a measurement. Additional detector artifacts are removed[8] by subtracting a cross-correlation matrix  $XC = (XT_{-1} + XT_{+1})/2$  from  $C(q, t_1, t_2, n)$ , where  $XT_{-1} = (X_{-1} + X_{-1}^T)/2$  and  $XT_{+1} = (X_{+1} + X_{+1}^T)/2$ .  $X_{-1}$  and  $X_{+1}$  are cross correlation matrices calculated between intensities in neighboring pulse trains according to  $X_{-1} = \frac{\langle \delta I_{n-1}(q, t_1) \delta I_n(q, t_2) \rangle_{\text{sp}}}{\langle I_{n-1}(q, t_1) \rangle_{\text{sp}} \langle I_n(q, t_2) \rangle_{\text{sp}}}$  and  $X_{+1} = \frac{\langle \delta I_n(q, t_1) \delta I_{n+1}(q, t_2) \rangle_{\text{sp}}}{\langle I_n(q, t_1) \rangle_{\text{sp}} \langle I_{n+1}(q, t_2) \rangle_{\text{sp}}}$ .  $C(q, t_1, t_2)$  is calculated by averaging  $C(q, t_1, t_2, n) - XC$  over the several hundred pulse trains,  $N$ , for each sample:  $C(q, t_1, t_2) = \frac{1}{N} \sum_{n=1}^N C(q, t_1, t_2, n) - XC$ .

The intensity-intensity autocorrelation function,  $g^{(2)}(q, \tau, \bar{t})$ , is calculated from  $C(q, t_1, t_2)$  via  $g^{(2)}(q, \tau, \bar{t}) - 1 = \overline{C(q, t_1, t_2)}$ , where  $\tau = t_2 - t_1$  and the overbar indicates an average over times  $t_1$  and  $t_2$  at constant average age,  $\bar{t}$ , where  $t = (t_1 + t_2)/2$ . We calculate intensity autocorrelation functions for different average ages,  $\bar{t}$ . We were not able to obtain useful autocorrelation functions at  $q$  values larger than  $\sim 0.030 \text{ \AA}^{-1}$  in the colloidal phase due to the decorrelation rates of the autocorrelation functions exceeding the instrumental limitation set by the X-ray pulse repetition rate of 2.2 MHz. We were unable to obtain meaningful autocorrelation functions for the liquid phase at higher  $q$  values due to the  $q^{-4}$  fall-off in signal strength. The autocorrelation functions are fit to the equation  $g^{(2)}(q, \tau, \bar{t}) - 1 = \beta(q) \exp[-2\Gamma(q, \bar{t})\tau]$ , where  $\beta(q)$  is the speckle contrast and  $\Gamma(q, \bar{t})$  is the rate at which the autocorrelation function decays.  $\beta(q)$  in the fits in **Figure 3** is fixed based on the average of the direct calculation of the speckle contrast, i.e.,  $C(q, t_1, t_1)$ , of hundreds of individual images (see **Figure S11**). We do not fit a stretched exponential function to the autocorrelation functions of the colloidal phase so as not to overfit the data, given the fast time scales of the decorrelation relative to the time between X-ray pulses in a pulse train. If we fit a stretched exponential to the autocorrelation functions of the liquid phase, the stretching exponent obtained is  $\sim 1$ . We therefore fit a simple exponential to the autocorrelation functions of the liquid phase to aid in the analysis and comparison to the colloidal phase.

**Approximations for  $H^i(q)$ .** The hydrodynamic functions are extracted from the decorrelation rates via  $H_p^i(q) = \Gamma^i(q, \bar{t} \rightarrow 0)S^i(q)/D_0q^2$ , where  $\Gamma^i(q, \bar{t} \rightarrow 0)$  are the rates at which the autocorrelation functions decay,  $D_0$  is the bare self-diffusion coefficient of dilute NCs,  $S^i(q)$  are the structure factors, and  $i = c, \ell$  for the colloidal and liquid phases, respectively. The hydrodynamic functions of a polydisperse sample,  $H_p^i(q)$ , are related to the hydrodynamic functions of an idealized monodisperse sample,  $H^i(q)$ , via  $H_p^i(q) = [1 - X_p(q)]\frac{D_s}{D_0} + X_p(q)H^i(q)$ , where  $D_s$  is the self-diffusion coefficient of the NCs in the system.[24] Since  $X_p(q) \sim 1$  in the  $q$ -range we performed the correlation analysis (**Figure S12**), we treat  $H_p^i(q)$  as  $H^i(q)$ . Because we only extract  $H^i(q)$  over a limited  $q$  range in the experiments (**Figure 4a** in the main text), we cannot use the  $q \sim 0.3 \text{ \AA}^{-1}$  value of  $H^i(q)$  to approximate  $D_s/D_0$ .  $H^\ell(q)$  will oscillate at  $q$  values larger than  $\sim 0.3 \text{ \AA}^{-1}$  due to the peak in the structure factor,  $S^\ell(q)$ . Because of this fact, we turn to the approximation method described below and Brownian dynamics simulations to extract the  $q \rightarrow \infty$  limit of  $H^i(q)$ , i.e.,  $D_s/D_0$ .

The hydrodynamic functions are also given by

$$H^i(q) = \frac{1}{ND_0q^2} \left\langle \sum_{m,n=1}^N \mathbf{q} \cdot \mathbf{D}_{mn}^i \cdot \mathbf{q} \exp[i\mathbf{q} \cdot (\mathbf{r}_m - \mathbf{r}_n)] \right\rangle,$$

where  $\mathbf{D}_{mn}^i$  is a diffusivity tensor that relates the hydrodynamic force on NC  $n$  to the translational velocity of NC  $m$ . [15] We split  $H^i(q)$  into self ( $D_s^i/D_0$ ) and distinct ( $H_d^i(q)$ ) parts, where  $i=c, \ell$ . The  $\delta\gamma$ -method of Beenakker and Mazur to approximate  $H^i(q)$  is an effective medium approach based on a partial resummation of many body hydrodynamic interactions. [5, 4, 9] In the standard application of this method,  $D_s^i/D_0 = \frac{2}{\pi} \int_0^\infty dy [\frac{\sin y}{y}]^2 [1 + \phi^i S_{\gamma 0}(y)]^{-1}$ , where  $y = q\sigma$ ,  $\sigma$  is the diameter of the NCs,  $\phi^i$  is the volume fraction of NCs in phase  $i$ ,  $S_{\gamma 0}(y) = \frac{9}{2} [\text{Si}(2y)y^{-1} + \frac{1}{2} \cos(2y)y^{-2} + \frac{1}{4} \sin(2y)y^{-3} - (\sin y)^2 y^{-4} - 4(\sin y - y \cos y)^2 y^{-6}]$ , and  $\text{Si}(2y) = \int_0^{2y} dt \sin t/t$ .  $H_d^i(q) = \frac{3}{2\pi} \int_0^\infty dy' [\frac{\sin y'}{y'}]^2 [1 + \phi^i S_{\gamma 0}(y')]^{-1} \int_{-1}^1 d\mu (1 - \mu^2) [S^i(|\mathbf{q} - \mathbf{q}'|) - 1]$ , where  $\mu$  is the cosine of the angle between  $\mathbf{q}$  and  $\mathbf{q}'$ . The only input to these equations is the volume fraction of NCs,  $\phi^i$ , and the structure factors,  $S^i(q)$ . Higher order corrections to these approximations would require higher order correlation functions as input. The  $\delta\gamma$ -method overestimates  $D_s^\ell/D_0$ , so we instead fit the  $\delta\gamma$ -method prediction for  $H_d^\ell(q)$  plus a constant offset to the  $H^\ell(q)$  values extracted from experiment to obtain the blue curve in **Figure 4a**. The value of the constant, which is equal to  $D_s^\ell/D_0$ , is 0.23.

**Brownian dynamics simulations.** Simulations of NCs were performed with an underdamped Langevin dynamics in the  $NVT$  ensemble in a cubic periodic box using the LAMMPS software. [21] NCs were represented as 4000 spherical particles with pairwise interactions given by a Lennard-Jones potential:  $u_{\text{LJ}}(r) = 4\epsilon[(\sigma/r)^{12} - (\sigma/r)^6]$ , where  $\epsilon$  is the depth of the interaction potential,  $\sigma$  is the diameter of the NCs, and  $r$  is the center-to-center distance between the NCs. At a given temperature  $T$ , the diffusive time scale for NCs is given by  $t_0 = \gamma\sigma^2/k_B T$  where  $\gamma$  is the friction coefficient in Langevin dynamics, and  $k_B$  is Boltzmann's constant. We have chosen the density of NCs in the simulation box, mass of NCs, temperature, friction coefficient, and simulation time step as  $0.1/\sigma^3$ ,  $0.2\gamma^2\sigma^2/\epsilon_{\text{LJ}}$ ,  $\epsilon_{\text{LJ}}/k_B$ ,  $100m$  ( $m$ =mass), and  $1 \times 10^{-4}t_0$ , respectively.

The NCs are first equilibrated at  $\epsilon$  before calculating the expected coherent scattering patterns,  $S(\mathbf{q}, t)$ . From these values, autocorrelation functions,  $\langle S(\mathbf{q}, 0)S(\mathbf{q}, \tau) \rangle / \langle S(\mathbf{q}) \rangle^2$ , were calculated and fit to a stretched exponential function to extract  $\Gamma(q)$ .  $H(q)$  was extracted using the following equation:  $H(q) = \Gamma(q)S(q)/(D_0 q^2)$ , where  $D_0 = 0.0460\sigma^2/t_0$  and  $S(\mathbf{q}) = \frac{1}{N} |\sum_{n=1}^N e^{-i\mathbf{q} \cdot \mathbf{r}_n}|^2$ . Here,  $\mathbf{r}_n$  is the location of NC  $n$ ,  $N = 4000$ , and  $t_0$  is the diffusive time scale of NCs.

**Liquid droplet size.** We place a lower bound on the radius of gyration of the liquid droplets to be  $\sim 90$  nm, or  $\sim 30$  times larger than the NC radii. This bound is based on the smallest  $q$ -value measured in SAXS patterns of the liquid phase taken at synchrotrons (**Figure S13**) due to the limited  $q$ -range at MID. In the Guinier region ( $q \rightarrow 0$ ), the scattered intensity has the form  $I(q) = I_0 e^{-q^2 R_g^2/3}$ , where  $I_0$  is a constant and  $R_g$  is the average radius of gyration of the liquid droplets. At higher  $q$ -values in the Porod region, the scattered intensity scales as  $q^{-\text{pe}}$ , where  $\text{pe}$  is the Porod exponent (4 in this case). Moving from high  $q$  to low  $q$ , the scattered intensity will transition from the power law scaling to the exponential behavior and plateau for  $q$ -values at which  $qR_g < 1$ . The crossover between these two regions occurs at  $q \sim 2\pi/R_g$ . We do not observe any such crossover in the SAXS patterns of the NC liquid phase up to smallest measured  $q$ -value of  $0.0068 \text{ \AA}^{-1}$ . This observation enables us to place a lower bound on the radius of gyration of the liquid droplets to be  $\sim 2\pi/0.0068 \text{ \AA}^{-1} = 92$  nm.

**Time-dependent heating.** The decorrelation rates increase with  $\bar{t}$  due to the solvent

viscosity decreasing and the temperature of the solvent surrounding the NCs increasing. The decorrelation rate is related to the temperature via  $\Gamma(\bar{t}) = D(\bar{t})q^2 = k_B T(\bar{t})q^2 / 6\pi\eta(T)R_H$  where  $D(\bar{t})$  is the diffusion coefficient of NCs in the colloidal phase,  $k_B$  is Boltzmann's constant,  $\eta(T)$  is the solvent viscosity, and  $R_H$  is the hydrodynamic radius of the NCs. Based on the DLS experiments shown in **Figure S6**, we set  $R_H$  to 3.2 nm.

The temperature of the solvent after the absorption of  $n$  X-ray pulses in a pulse train of  $N = 50$  total pulses is [13, 7]  $T_{\text{solv}}(n) = \Delta T_{\text{solv}} \sum_{n=0}^N \frac{1}{1+(n\tau_0/\tau_1)} + T_0$ , where  $T_0 = 300$  K is the initial temperature,  $\tau_0 = 443$  ns is the time between two pulses in a pulse train,  $\tau_1$  is the characteristic time with which the heated probe volume equilibrates its temperature with the surrounding sample, and  $\Delta T_{\text{solv}}$  is the instantaneous temperature jump of the solvent due to X-ray absorption. Here,  $\tau_1 = \frac{c_p \rho_{\text{solv}} \sigma_b^2}{2K_{\text{solv}}}$ , where  $c_p = 2.12$  J/(g K) is the solvent heat capacity,  $\rho = 985800$  g/m<sup>3</sup> is the solvent density,  $\sigma_b$  is the X-ray beam size, and  $K_{\text{solv}} = 0.1962$  W/(m K) is the thermal conductivity of the solvent. The X-ray beam size is  $\sim 1\text{-}2$   $\mu\text{m}$  (**Figure S9**). With these parameters, we obtain  $\tau_1 = 64$   $\mu\text{s}$ . In addition,  $\Delta T_{\text{solv}} = \frac{E_{\text{pulse}}/\sigma_b^2}{2\pi c_p \rho_{\text{solv}} \lambda_{\text{abs}}/[4 \ln 2]}$ . Here,  $\lambda_{\text{abs}} = 6$   $\mu\text{m}$  is the solvent absorption length for 12.3 keV X-rays and  $E_{\text{pulse}}$  is the energy of the X-rays incident on the sample. We estimate  $\sim 2$   $\mu\text{J}$ /pulse is incident on the sample based on the energies of the X-ray pulses and the expected losses through the beamline optics. The result of this calculation of the temperature of the solvent due to X-ray absorption is shown in **Figure S8a** (black curve).

The temperature of the solvent surrounding a NC following the absorption of X-rays is [13, 7]  $\Delta T_{\text{ss}}(r, t) = \frac{(\Delta T_{\text{NC}}) \exp[-3 \frac{K_{\text{NC}}}{K_{\text{solv}}} Bi \frac{\alpha}{R^2} t]}{r/R}$ , where  $r$  is the distance from the NC,  $R$  is the NC radius,  $t$  is the time after the X-rays are absorbed,  $\Delta T_{\text{NC}}$  is the temperature of a NC immediately after X-ray absorption,  $K_{\text{NC}} = 2.19$  W/(m K) is the NC heat conductivity,  $\alpha = \frac{K_{\text{NC}}}{\rho c_p^{\text{NC}}}$ ,  $c_p^{\text{NC}} = 49.5$  J/(mol K) is the NC heat capacity,  $Bi = hR/K_{\text{NC}}$  is the Biot number,  $h$  is the convective heat transfer coefficient. The convective heat transfer coefficient is not known for the PbS NC interface with NMF/DMF solvent due to difficulties measuring heat flow on the nanoscale, but we use a value of  $4.7 \times 10^3$  J/(s m<sup>2</sup>K) for the calculations in this work. The result of this calculation for the temperature profile 2 nm from the NC surface is shown in **Figure S6a** (red curve).

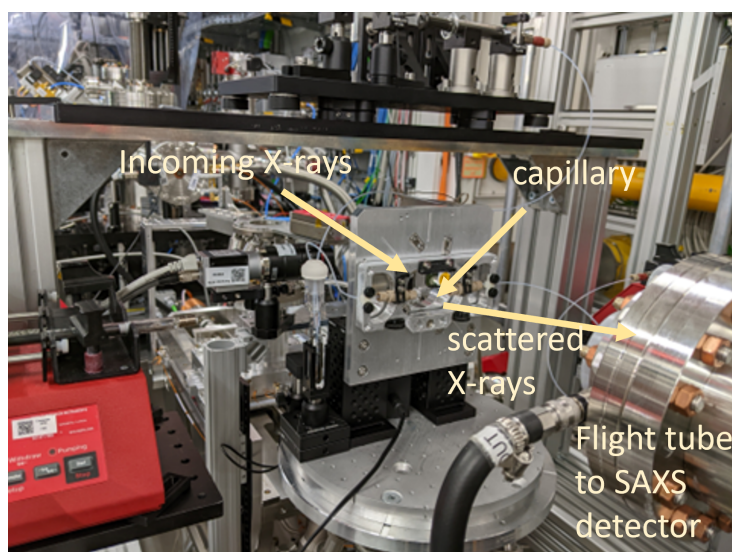

**Figure S1. Experimental setup at the MID instrument at the EuXFEL.** Incoming X-ray pulse trains are incident upon the sample held in a horizontally mounted capillary. Scattered X-rays enter the flight tube to the SAXS detector located 7 m downstream of the sample.

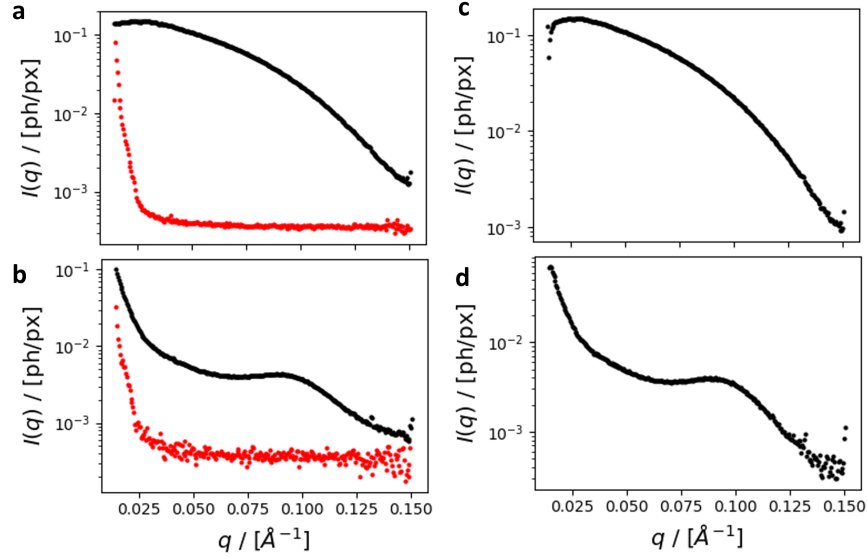

**Figure S2. Background subtraction of SAXS patterns.** **a.** Train-averaged SAXS pattern taken from a glass capillary of colloidal NCs dispersed in a 60/40 mixture of N-methylformamide (NMF)/N,N-dimethylformamide (DMF) (black points) and a glass capillary filled with a 60/40 mixture of NMF/DMF (red points). **b.** Train-averaged SAXS pattern taken from a glass capillary of NCs dispersed in a 60/40 mixture of NMF/DMF with 170 mM  $K_3AsS_4$  salt (black points) and a glass capillary filled with a 60/40 mixture of NMF/DMF with 170 mM  $K_3AsS_4$  salt (red points). **c.** Subtraction of background (red points) from data (black points) in **a**. **d.** Subtraction of background (red points) from data (black points) in **b**.

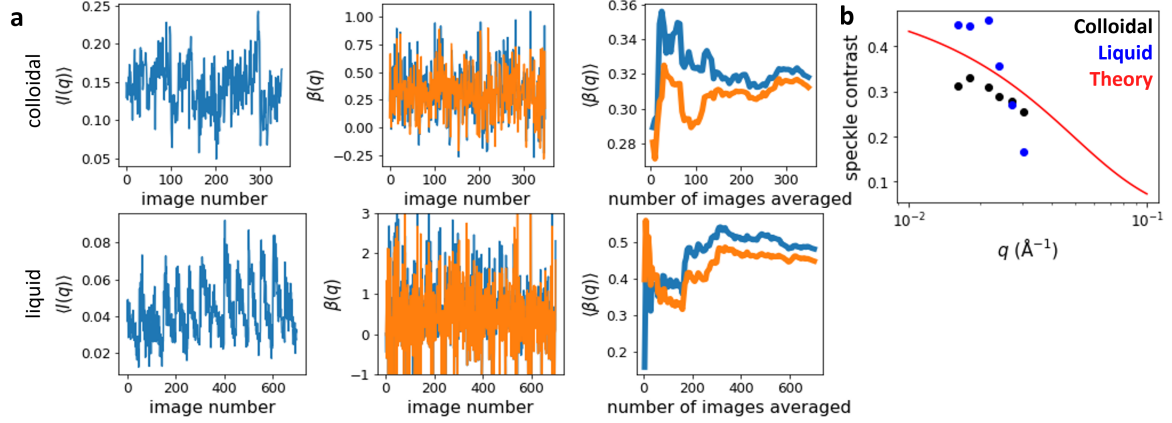

**Figure S3. Calculation of speckle contrast from individual detector images. a.** The spatially averaged detector intensity for the region of interest (ROI) centered on  $q=0.016 \text{ \AA}^{-1}$  for a series of images in units of photons per pixel (left), speckle contrast  $\beta(q)$  of each corresponding image (middle), and average speckle contrast based on an increasing number of images used in the average (right) for the colloidal sample (top row) and liquid sample (bottom row). The speckle contrasts converge in a similar manner for the other ROIs. The converged values of  $\langle\beta(q)\rangle$  are used to constrain the value of the autocorrelation functions at  $\tau=0$  in the fits in **Figure 3** and **Figure S4**. Blue curves in the middle and right hand columns are speckle contrasts calculated via  $\beta(q) = \frac{2\tilde{P}(2)[1-\tilde{P}(1)]}{\tilde{P}(1)^2} - 1$ , where  $\tilde{P}(k)$  is the probability of observing  $k$  photons per pixel in a detector image.[10] Orange curves in the middle and right hand columns are speckle contrasts calculated via  $\beta(q) = \frac{\langle I(q)^2 \rangle - \langle I(q) \rangle^2}{\langle I(q) \rangle^2} - \frac{1}{\langle I(q) \rangle}$ , where  $\langle I(q) \rangle$  is the average number of photons per pixel at wavevector  $q$ . [13] These two methods converge on similar values of  $\beta(q)$  as more images are used in the average. **b.** The average speckle contrast as a function of  $q$  for the colloidal (black points) and liquid (blue points) phases. The red curve is the predicted dependence of the speckle contrast based on the geometry of the experimental setup. Specifically, the red curve,  $\beta_{\text{Th}}$ , is given by  $\beta_{\text{Th}} = \beta_{\text{cl}}\beta_{\text{res}}$  [14]. The contrast due to the finite angular resolution of the experiment,  $\beta_{\text{res}}$ , is given by  $\beta_{\text{res}} = \left\{ \frac{2}{w^2} \int_0^w (w - \nu) \frac{\sin \nu/2}{\nu/2} d\nu \right\}^2$ , where  $w = 2\pi Pa/d_{\text{S-D}}\lambda$ ,  $P = 200 \text{ }\mu\text{m}$  is the pixel size,  $a$  is the beam size,  $\lambda$  is the X-ray photon wavelength, and  $d_{\text{S-D}} = 7 \text{ m}$  is the sample-to-detector distance. The contrast due to the finite coherence lengths of the beam,  $\beta_{\text{cl}}$  is given by  $\beta_{\text{cl}} = \frac{2}{(ad)^2} \int_0^a dx \int_0^d dz (a-x)(d-z) \exp(-x^2/\xi^2) [\exp(-2|Ax+Bz|) + \exp(-2|Ax-Bz|)]$ , where  $A = (\Delta\lambda/\lambda)q\sqrt{1 - q^2/4k^2}$ ,  $B = -(\Delta\lambda/2\lambda)q^2/k$ ,  $k = 2\pi/\lambda$ ,  $d = 0.9 \text{ mm}$  is the sample thickness,  $\xi$  is the transverse coherence length of the beam that we take to be equal to the beam size, and  $\Delta\lambda/\lambda = 8 \times 10^{-4}$  is the bandwidth of the X-ray beam. We use a beam size of  $a = 4 \text{ }\mu\text{m}$  to obtain the red curve (see **Figure S9** for other methods of estimating the beam size). We attribute the difference between the contrast in the colloidal and liquid samples to be due to differences in the ratio of coherent scattering to incoherent background scattering in the different experiments.

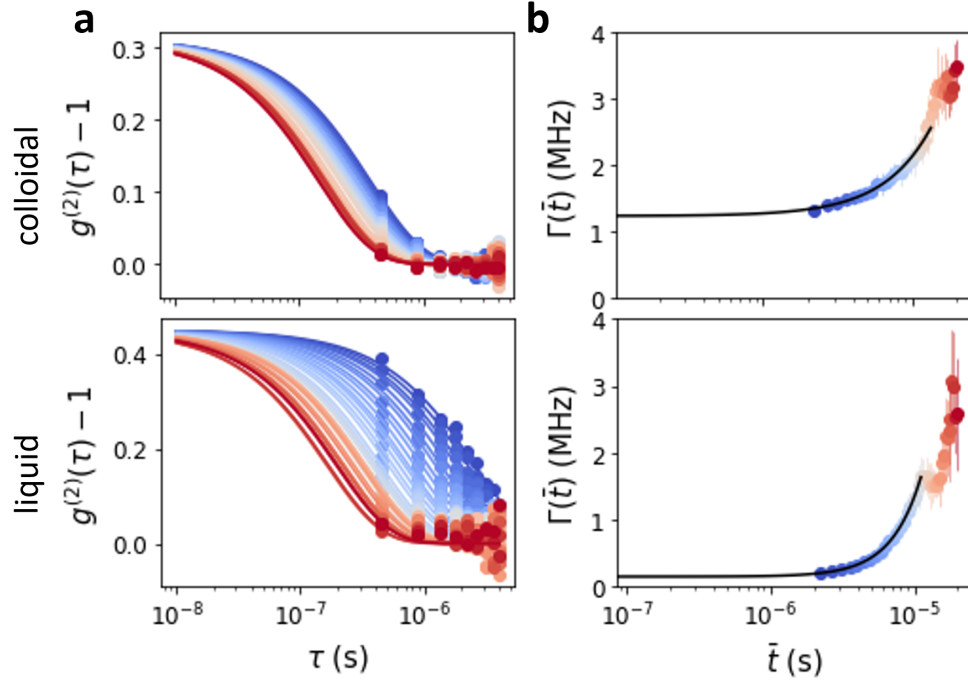

**Figure S4. Autocorrelation functions change during the pulse trains.** **a.** Autocorrelation functions at  $q=0.016 \text{ \AA}^{-1}$  as a function of  $\bar{t}$  (blue and red points) for NCs in the colloidal phase (top) and liquid phase (bottom). Here,  $\bar{t}$  increases from blue to red from  $2.2 \mu\text{s}$  to  $19.5 \mu\text{s}$  in steps of  $0.43 \mu\text{s}$ . Solid curves are exponential fits constrained at  $\tau = 0$  by  $0.312$  and  $0.449$  for the colloidal and liquid phases, respectively (see **Figure S8**). **b.** Decorrelation rate,  $\Gamma$ , as a function of  $\bar{t}$  for the exponential fits in **a**. Colors same as in **a**. Black curves indicate power law fits ( $\Gamma(\bar{t}) = a\bar{t}^b + c$ ). We use the best-fit value of the parameter  $c$  as an estimate for the decorrelation rate of the unperturbed NC dynamics (closed black and blue circles in **Figure 3c** in the main text).

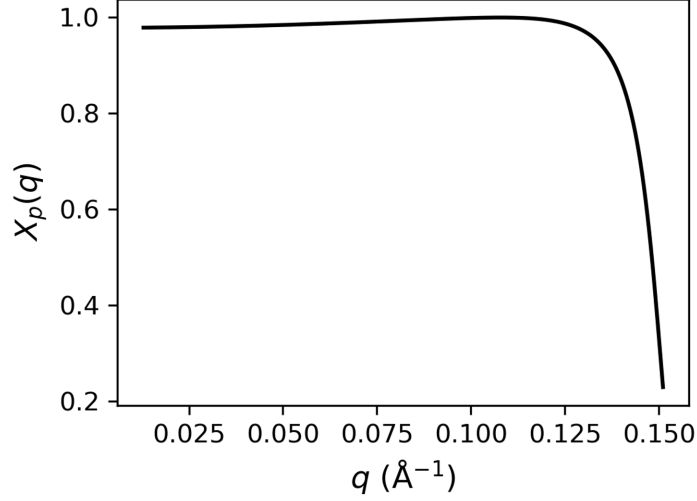

**Figure S5. Decoupling amplitude.** The decoupling amplitude,  $X_p(q)$ , for the NCs based on the best-fit NC radius (excluding the ligands) of 2.89 nm from the fit in main text **Figure 2b**. We use a polydispersity of 5% based on fits to SAXS patterns taken at synchrotrons with larger  $q$ -ranges than at MID.[20]

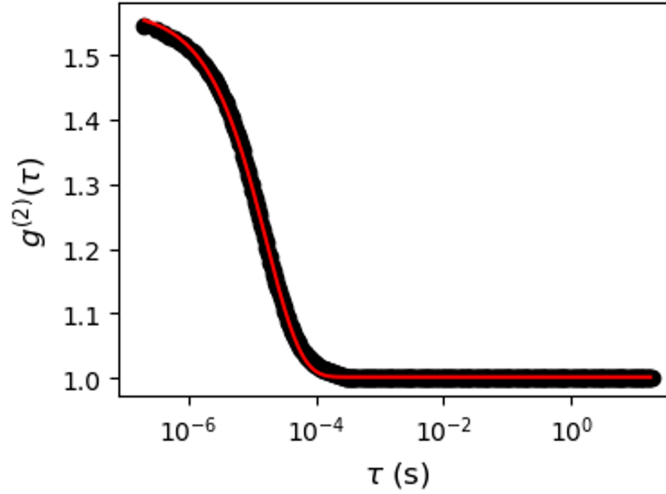

**Figure S6. Autocorrelation function of colloidal NCs measured via dynamic light scattering (DLS).** Autocorrelation function (black points) and exponential fit (red curve) for colloidal PbS NCs dispersed in a 60/40 mixture of NMF/DMF at a volume fraction of 0.0002. The measurement was made on a Wyatt Technology instrument with a laser wavelength of 532 nm and the scattered intensity was recorded at 163.5°. The decorrelation rate of  $\sim 30$  kHz corresponds to a diffusion coefficient of  $55 \mu\text{m}^2/\text{s}$  or a hydrodynamic diameter of 6.4 nm. We take  $55 \mu\text{m}^2/\text{s}$  to be  $D_0$ .

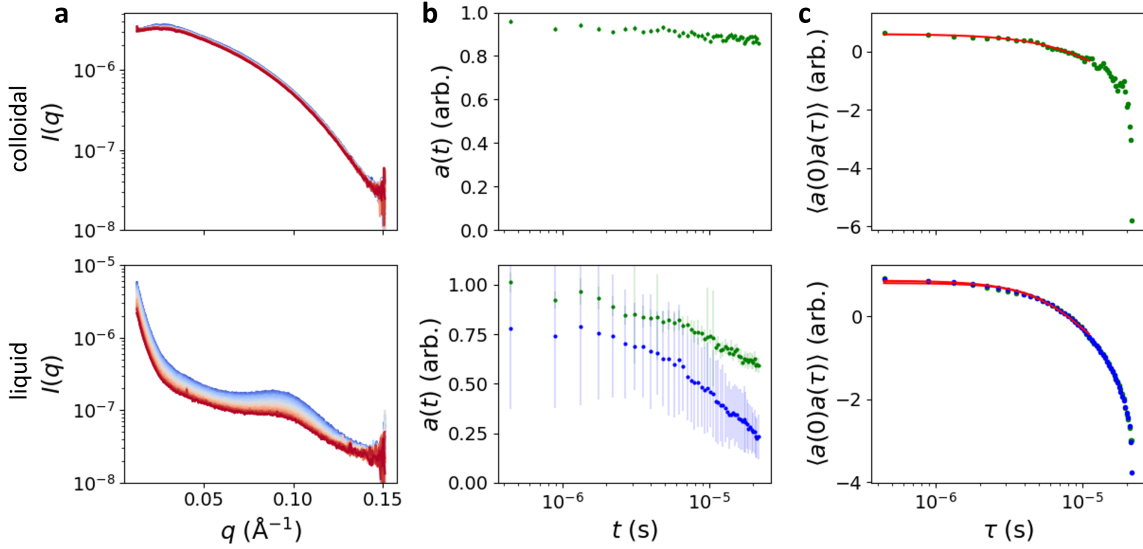

**Figure S7. Time scale of NCs exiting the X-ray probe volume.** **a.** Train-averaged SAXS patterns as a function of X-ray pulse location within each pulse train for a colloidal sample (top) and liquid sample (bottom). Solid curves represent the average over all trains of the SAXS patterns resulting from the  $n$ th pulse within the 50-pulse X-ray pulse train, where  $n$  goes from 1 to 50. Pulse number  $n$  increases from blue to red. Each SAXS pattern is fit to the same model used to fit the SAXS patterns in **Figure 2b** of the main text. **b.** The time dependence of the colloidal (green) and liquid (blue) components of the SAXS model. **c.** Autocorrelation of the concentration fluctuations of NCs in the colloidal (green) and liquid (blue) phases. Exponential fits are shown in red curves. The rate at which the concentration fluctuations decorrelate is  $\sim 0.07$  MHz for the NCs in the colloidal phase (top) and  $\sim 0.09$  MHz for NCs in the liquid phase (bottom). These decorrelation rates corresponding to the time scale on which NCs leave the probe volume due to heating effects are much slower than the decorrelation rates of interest for the NCs in the colloidal and liquid phases.

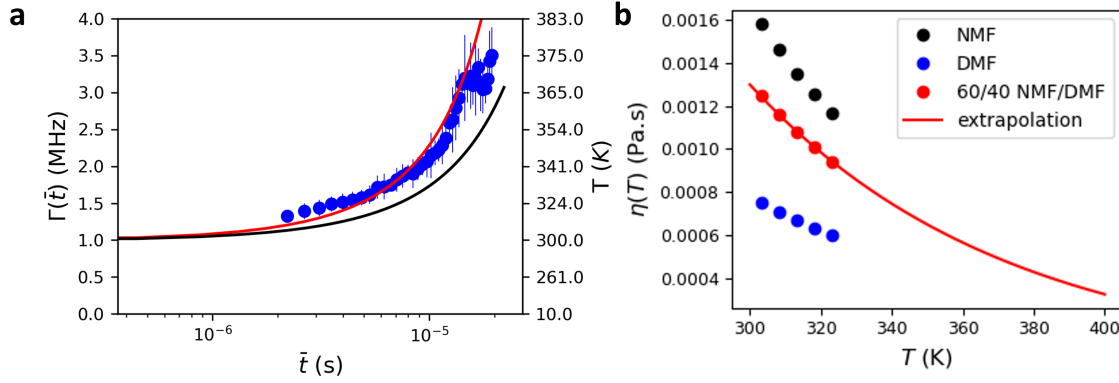

**Figure S8. Time-dependent heating.** **a.** Decorrelation rate,  $\Gamma$ , and temperature,  $T$ , of NCs in the colloidal phase as a function of average age in the pulse train,  $\bar{t}$ , for the smallest  $q$ -value shown in main text **Figure 3**. The black curve denotes the temperature profile of the NCs predicted from solvent heating. The red curve denotes the decorrelation rate of the NCs as the temperature of the solvent surrounding the NCs increases with increased X-ray pulse exposure. Calculations are performed as in references ([13, 8]) and are described above. **b.** Temperature-dependent viscosity of N-methylformamide and N,N-dimethylformamide (data points) ([1]). The red points corresponding to the 60/40 mixture are 60/40 weighted average of the NMF and DMF points. The red curve indicates an extrapolation of the temperature-dependent viscosity of a 60/40 mixture of NMF/DMF based on an exponential fit.

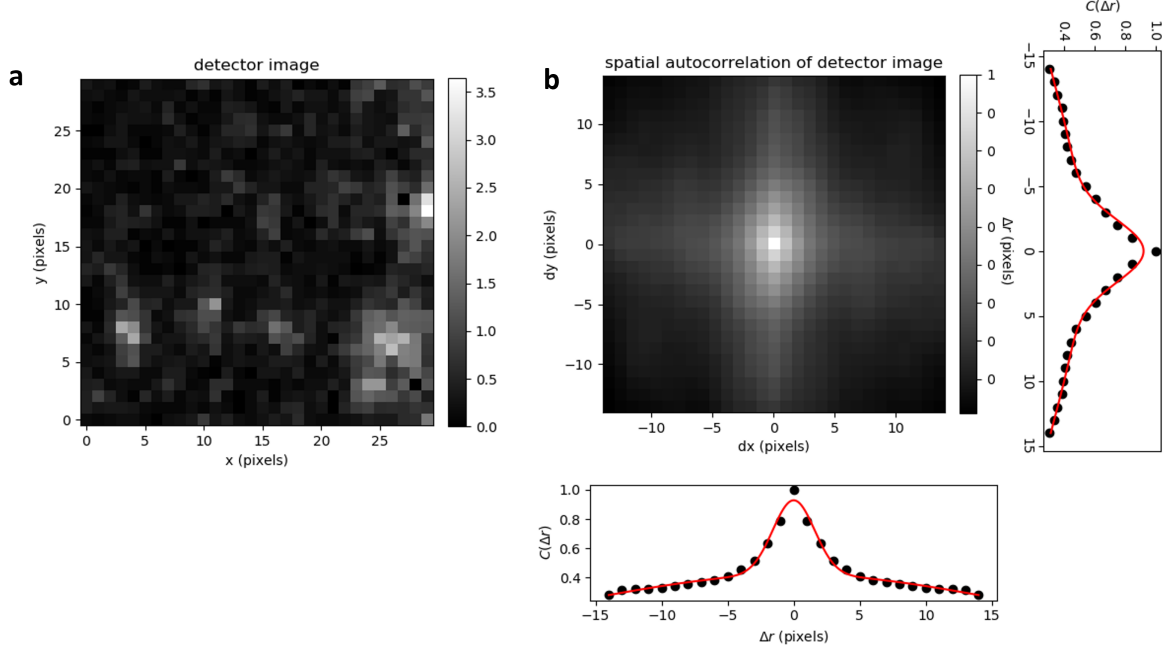

**Figure S9. X-ray beam size.** **a.** Image of speckles on the AGIPD. **b.** Unnormalized spatial autocorrelation,  $C(dx, dy)$  of detector image in **a**. Slices of  $C(dx, dy)$  are shown as insets:  $C(dx, dy = 0)$  (horizontal inset) and  $C(dx = 0, dy)$  (vertical inset). Red curves are Gaussian fits to the slices, with a best fit full width at half maximum (FWHM) of  $h=3.3$  pixels and  $v=6.8$  pixels (each pixel is  $200 \mu\text{m} \times 200 \mu\text{m}$  and  $h$  and  $v$  indicate the FWHM of horizontal and vertical slices of  $C(dx, dy)$ , respectively). This speckle size translates to an X-ray beam size of  $0.85\lambda d_{\text{S-D}}/s \sim 1 \mu\text{m}$ , where  $s = \sqrt{(\pi/4)hv}$  is the speckle size,  $\lambda$  is the X-ray wavelength, and  $d_{\text{S-D}}$  is the sample-detector distance (7 m) ([18, 25]).

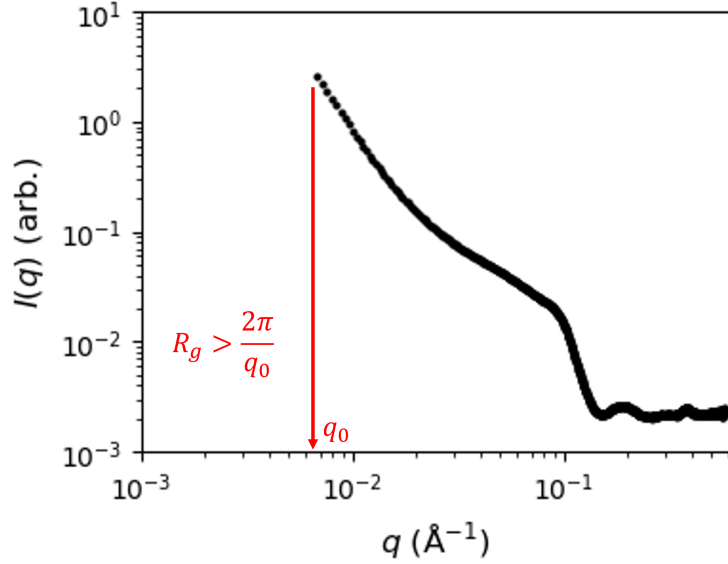

**Figure S10. Liquid droplet size estimate.** A SAXS pattern of the NC liquid state taken at a synchrotron (Advanced Light Source, beamline 7.3.3) with the minimum  $q$ -value,  $q_0$ , of  $0.0068 \text{ \AA}^{-1}$  suggests a lower bound on the liquid droplet size of  $R_g$  of  $\sim 90 \text{ nm}$ .

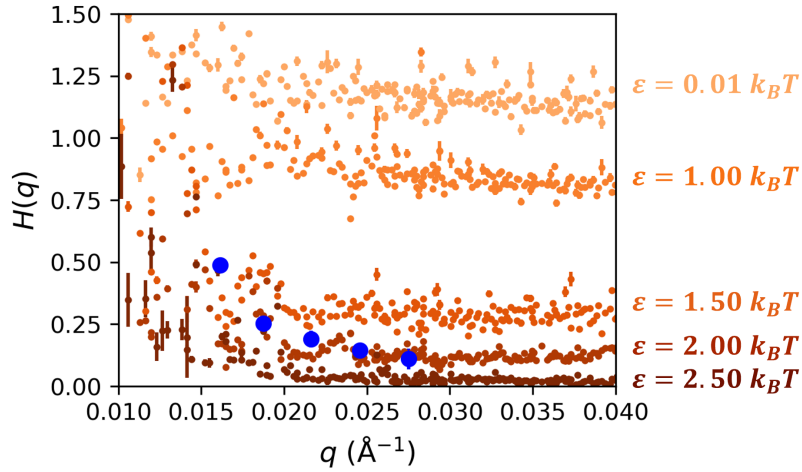

**Figure S11.**  $H(q)$  obtained from Brownian dynamics simulations.  $H(q)$  of NCs in the liquid phase extracted from experiments (blue) and  $H(q)$  extracted from Brownian dynamics simulations of NCs interacting with different well depths,  $\epsilon$ , in orange/brown shades.

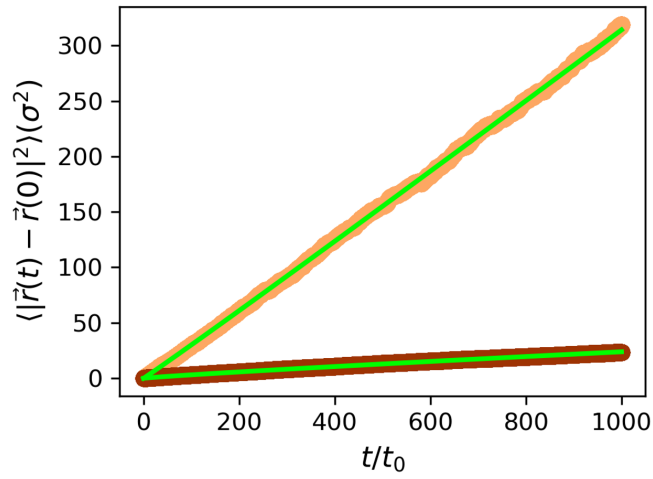

**Figure S12.** Mean-squared displacement (MSD) of NCs in the Brownian dynamics simulations. MSD of NCs interacting with a well depth  $\epsilon = 0.01 k_B T$  at a volume fraction of 0.007, i.e., in the colloidal phase (orange points), and  $\epsilon = 2 k_B T$ , i.e., in the liquid phase (brown points). Green lines are fits to  $MSD = 6D_s t$ , where  $D_s$  is the self-diffusion coefficient of the NCs in the simulations. The best-fit values of  $D_s$  are  $0.0460$  and  $0.0185 \sigma^2/t_0$  for the NCs in the colloidal and liquid phases, respectively. We take  $D_s = 0.046 \sigma^2/t_0$  to be  $D_0$ . See main text for definitions of  $\sigma$  and  $t_0$ .

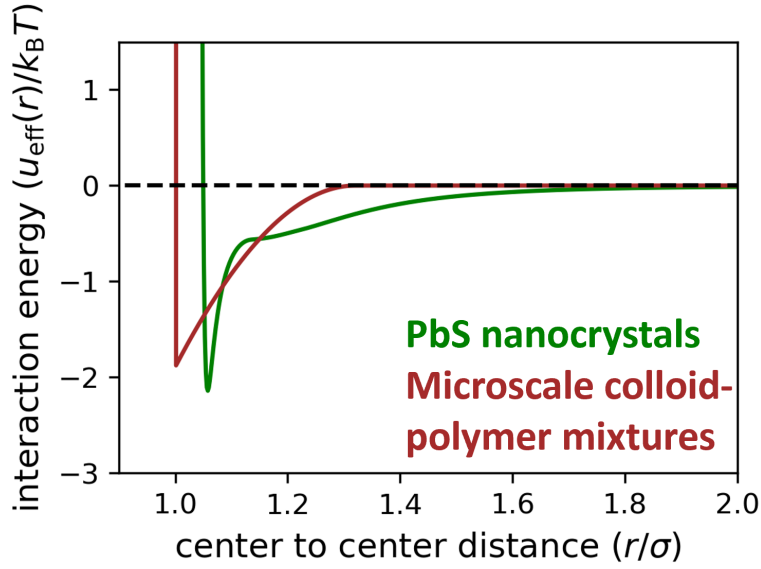

**Figure S13.** Interparticle interactions of PbS NCs and microscale colloid-polymer mixtures. The PbS NC interactions are calculated using DLVO theory[11] and the Asakura-Oosawa model[2, 3, 22] to account for the depletion interaction of the finite-sized salt ions and solvent molecules. The colloid-polymer mixture interactions are calculated using the Asakura-Oosawa model at a polymer-particle size ratio,  $\xi$ , of 0.32 and a polymer free volume fraction of 0.33, which are the values of the system whose dynamics are shown in brown points in **Figure 4b** in the main text.[17] The interparticle potentials are plotted as a function of center-to-center distance between the NCs and colloidal particles, respectively. These distances are normalized by the size,  $\sigma$ , of the particles.

## References

- [1] Shamim Akhtar, A. N. M. Omar Faruk, and M. A. Saleh. Viscosity of Aqueous Solutions of Formamide, N-Methylformamide and N,N-Dimethylformamide. *Physics and Chemistry of Liquids*, 39(3):383–399, May 2001. Publisher: Taylor & Francis \_eprint: <https://doi.org/10.1080/00319100108031670>.
- [2] Sho Asakura and Fumio Oosawa. On Interaction between Two Bodies Immersed in a Solution of Macromolecules. *The Journal of Chemical Physics*, 22(7):1255–1256, July 1954.
- [3] Sho Asakura and Fumio Oosawa. Interaction between particles suspended in solutions of macromolecules. *Journal of Polymer Science*, 33(126):183–192, 1958.
- [4] C. W. J. Beenakker and P. Mazur. Diffusion of spheres in a concentrated suspension II. *Physica A: Statistical Mechanics and its Applications*, 126(3):349–370, July 1984.
- [5] C.W.J. Beenakker and P. Mazur. Self-diffusion of spheres in a concentrated suspension. *Physica A: Statistical Mechanics and its Applications*, 120(3):388–410, July 1983.
- [6] Igor Coropceanu, Eric M. Janke, Joshua Portner, Danny Haubold, Trung Dac Nguyen, Avishek Das, Christian P. N. Tanner, James K. Utterback, Samuel W. Teitelbaum, Margaret H. Hudson, Nivedina A. Sarma, Alex M. Hinkle, Christopher J. Tassone, Alexander Eychmüller, David T. Limmer, Monica Olvera de la Cruz, Naomi S. Ginsberg, and Dmitri V. Talapin. Self-assembly of Nanocrystals into Strongly Electronically Coupled All-Inorganic Supercrystals. *Science*, 375(6587):1422–1426, March 2022.
- [7] F. Dallari, A. Jain, M. Sikorski, J. Möller, R. Bean, U. Boesenberg, L. Frenzel, C. Goy, J. Hallmann, Y. Kim, I. Lokteva, V. Markmann, G. Mills, A. Rodriguez-Fernandez, W. Roseker, M. Scholz, R. Shayduk, P. Vagovic, M. Walther, F. Westermeier, A. Madsen, A. P. Mancuso, G. Grübel, and F. Lehmkuhler. Microsecond hydrodynamic interactions in dense colloidal dispersions probed at the European XFEL. *IUCrJ*, 8(5):775–783, September 2021. Publisher: International Union of Crystallography.
- [8] Francesco Dallari, Mario Reiser, Irina Lokteva, Avni Jain, Johannes Möller, Markus Scholz, Anders Madsen, Gerhard Grübel, Fivos Perakis, and Felix Lehmkuhler. Analysis Strategies for MHz XPCS at the European XFEL. *Applied Sciences*, 11(17):8037, January 2021. Number: 17 Publisher: Multidisciplinary Digital Publishing Institute.
- [9] Marco Heinen, Adolfo J. Banchio, and Gerhard Nägele. Short-time rheology and diffusion in suspensions of Yukawa-type colloidal particles. *The Journal of Chemical Physics*, 135(15):154504, October 2011.
- [10] S. O. Hruszkewycz, M. Sutton, P. H. Fuoss, B. Adams, S. Rosenkranz, K. F. Ludwig, W. Roseker, D. Fritz, M. Cammarata, D. Zhu, S. Lee, H. Lemke, C. Gutt, A. Robert, G. Grübel, and G. B. Stephenson. High Contrast X-ray Speckle from Atomic-Scale Order in Liquids and Glasses. *Physical Review Letters*, 109(18):185502, November 2012. Publisher: American Physical Society.

- [11] Jacob Israelachvili. *Intermolecular and Surface Forces*. Elsevier, Inc., third edition, 2011.
- [12] David J. Kinning and Edwin L. Thomas. Hard-sphere interactions between spherical domains in diblock copolymers. *Macromolecules*, 17(9):1712–1718, September 1984.
- [13] Felix Lehmkuhler, Francesco Dallari, Avni Jain, Marcin Sikorski, Johannes Möller, Lara Frenzel, Irina Lokteva, Grant Mills, Michael Walther, Harald Sinn, Florian Schulz, Michael Dartsch, Verena Markmann, Richard Bean, Yoonhee Kim, Patrik Vagovic, Anders Madsen, Adrian P. Mancuso, and Gerhard Grübel. Emergence of anomalous dynamics in soft matter probed at the European XFEL. *Proceedings of the National Academy of Sciences*, 117(39):24110–24116, September 2020. Publisher: Proceedings of the National Academy of Sciences.
- [14] J. Möller, M. Sprung, A. Madsen, and C. Gutt. X-ray photon correlation spectroscopy of protein dynamics at nearly diffraction-limited storage rings. *IUCrJ*, 6(5):794–803, September 2019. Publisher: International Union of Crystallography.
- [15] Gerhard Nägele. On the dynamics and structure of charge-stabilized suspensions. *Physics Reports*, 272(5):215–372, July 1996.
- [16] Jerome K. Percus and George J. Yevick. Analysis of Classical Statistical Mechanics by Means of Collective Coordinates. *Physical Review*, 110(1):1–13, April 1958. Publisher: American Physical Society.
- [17] Kurt F. Seefeldt and Michael J. Solomon. Self-diffusion in dilute colloidal suspensions with attractive potential interactions. *Physical Review E*, 67(5):050402, May 2003.
- [18] M. Sikorski, S. Song, A. Schropp, F. Seiboth, Y. Feng, R. Alonso-Mori, M. Chollet, H. T. Lemke, D. Sokaras, T.-C. Weng, W. Zhang, A. Robert, and D. Zhu. Focus characterization at an X-ray free-electron laser by coherent scattering and speckle analysis. *Journal of Synchrotron Radiation*, 22(3):599–605, May 2015. Publisher: International Union of Crystallography.
- [19] Christian P. N. Tanner, James K. Utterback, Joshua Portner, Igor Coropceanu, Avishek Das, Christopher J. Tassone, Samuel W. Teitelbaum, David T. Limmer, Dmitri V. Talapin, and Naomi S. Ginsberg. In Situ X-ray Scattering Reveals Coarsening Rates of Superlattices Self-Assembled from Electrostatically Stabilized Metal Nanocrystals Depend Nonmonotonically on Driving Force. *ACS Nano*, 18(7):5778–5789, February 2024. Publisher: American Chemical Society.
- [20] Christian P. N. Tanner, Vivian R. K. Wall, Joshua Portner, Ahhyun Jeong, Avishek Das, James K. Utterback, Leo M. Hamerlynck, Jonathan G. Raybin, Matthew J. Hurley, Nicholas Leonard, Rebecca B. Wai, Jenna A. Tan, Mumtaz Gababa, Chenhui Zhu, Eric Schaible, Christopher J. Tassone, David T. Limmer, Samuel W. Teitelbaum, Dmitri V. Talapin, and Naomi S. Ginsberg. Enhancing nanocrystal superlattice self-assembly near a metastable liquid binodal, April 2024. arXiv:2404.16808 [cond-mat].

- [21] Aidan P. Thompson, H. Metin Aktulga, Richard Berger, Dan S. Bolintineanu, W. Michael Brown, Paul S. Crozier, Pieter J. in 't Veld, Axel Kohlmeyer, Stan G. Moore, Trung Dac Nguyen, Ray Shan, Mark J. Stevens, Julien Tranchida, Christian Trott, and Steven J. Plimpton. LAMMPS - a Flexible Simulation Tool for Particle-Based Materials Modeling at the Atomic, Meso, and Continuum Scales. *Computer Physics Communications*, 271:108171, February 2022.
- [22] A. Vrij. Polymers at Interfaces and the Interactions in Colloidal Dispersions. *Pure and Applied Chemistry*, 48(4):471–483, January 1976. Publisher: De Gruyter.
- [23] M. S. Wertheim. Exact Solution of the Percus-Yevick Integral Equation for Hard Spheres. *Physical Review Letters*, 10(8):321–323, April 1963. Publisher: American Physical Society.
- [24] Fabian Westermeier, Birgit Fischer, Wojciech Roseker, Gerhard Grübel, Gerhard Nägele, and Marco Heinen. Structure and short-time dynamics in concentrated suspensions of charged colloids. *The Journal of Chemical Physics*, 137(11):114504, September 2012.
- [25] Kyuseok Yun, Sungwon Kim, Dongjin Kim, Myungwoo Chung, Wonhyuk Jo, Hyerin Hwang, Daewoong Nam, Sangsoo Kim, Jangwoo Kim, Sang-Youn Park, Kyung Sook Kim, Changyong Song, Sooheyong Lee, and Hyunjung Kim. Coherence and pulse duration characterization of the PAL-XFEL in the hard X-ray regime. *Scientific Reports*, 9(1):3300, March 2019. Publisher: Nature Publishing Group.
